# Supplementary material for: Self-Sampling for Neural Point Cloud Consolidation
Source: arXiv:2008.06471 source file (2022-05-13)
Supplement: Supplementary file 1 [file 06_supp.tex]

\section{Supplementary Materials}

\input{figures/004 experiments/table/individual/fig}
